# Supplementary material for: Ultra-Reliable Short-Packet Communications: Half-Duplex or Full-Duplex Relaying?
Source: arXiv:1711.08199 source file (2017-11-22)
Supplement: Supplementary file 1 [file appendix.tex]

\section{Proof of Proposition 1}
From (\ref{app1}) and (\ref{CDF}), the term $\Psi_{\delta, \tau}$ can be calculated as
\begin{equation}
\begin{split}
{\Psi _{\delta ,\tau}} &\approx {\vartheta _{\tau}}\sqrt {{m_{\tau}}} \int_{{\zeta _{\delta ,\tau}}}^{{\xi _{\delta ,\tau}}} {{F_{{\gamma _{\delta ,\tau}}}}\left( x \right)}dx \\
& \approx 1 -  {{{\vartheta _{\tau}}\sqrt {{m_{\tau}}}{c_{\delta ,\tau}}} \over {2\sqrt {{a_{\delta ,\tau}}{b_{\delta ,\tau}}} }}\int\limits_{{{2\sqrt {{a_{\delta ,\tau }}{b_{\delta ,\tau}}} } \over {{c_{\delta ,\tau}}}}{\zeta _{\delta ,\tau}}}^{{{2\sqrt {{a_{\delta ,\tau}}{b_{\delta ,\tau}}} } \over {{c_{\delta ,\tau}}}}{\xi _{\delta ,\tau}}} {y\exp \left( { - {{{a_{\delta ,\tau}} + {b_{\delta ,\tau}}} \over {2\sqrt {{a_{\delta ,\tau}}{b_{\delta ,\tau}}} }}y} \right)} {K_1}\left( y \right)dy
\end{split}
\end{equation}
It seems intractable to solve the above integral and we thus first use a series representation of $\exp\left( x \right)  = \sum\limits_{k = 0}^\infty  {{{{x^k}} \over {k!}}} $ \cite[Eq. (1.211-1)]{Tableofintegral}. We can then further evaluate the term $\Psi_{\delta, \tau}$ as

\begin{equation}
\begin{split}
{\Psi _{\delta ,\tau}} &\approx 1-{{{\vartheta _{\tau}}\sqrt {{m_{\tau }}} {c_{\delta ,\tau}}} \over {2\sqrt {{a_{\delta ,\tau}}{b_{\delta ,\tau}}} }}\sum\limits_{k = 0}^\infty  {{{{{\left( { - {{{a_{\delta ,\tau}} + {b_{\delta ,\tau }}} \over {2\sqrt {{a_{\delta ,\tau}}{b_{\delta ,\tau}}} }}} \right)}^k}} \over {k!}}} \int\limits_{{{2\sqrt {{a_{\delta ,\tau}}{b_{\delta ,\tau}}} } \over {{c_{\delta ,\tau}}}}{\zeta _{\delta ,\tau}}}^{{{2\sqrt {{a_{\delta ,\tau}}{b_{\delta ,\tau}}} } \over {{c_{\delta ,\tau}}}}{\xi _{\delta ,\tau}}} {{y^{k + 1}}} {K_1}\left( y \right)dy.\\
\end{split}
\end{equation}
We then represent the function $y^{k+1} K_1\left(y\right)$ in terms of Meijer's G-function \cite[Eq. (9.34-3)]{Tableofintegral}. After some tedious mathematical manipulation, the above integral involving Meijer's G function can be solved by \cite{MG} and ${\Psi_{\delta ,\tau}}$ can be derived in the form of (\ref{generalterm}).
